# Supplementary material for: Hell is Paved with Good Intentions: The Intricate Relationship Between Cognitive Biases and Dark Patterns
Source: arXiv:2405.07378 source file (2024-05-12)
Supplement: Supplementary file 1 [file Appendix.tex]

\section{Codebook}\label{app:codebook}
This appendix covers all 52 codes that resulted from the open coding of the four focus groups.

\begin{table*}[b]
\centering

\begin{tabular}{p{.1\textwidth} p{.03\textwidth} p{.25\textwidth} p{.5\textwidth}}
\toprule
\multicolumn{1}{c}{\textbf{Category}} & \multicolumn{1}{c}{\textbf{No.}} & \multicolumn{1}{c}{\textbf{Code}} & \multicolumn{1}{c}{\textbf{Description}}\\ \hline

&  1.  & Awareness of a machine & Scenarios in which it is apparent that one interacts with a machine. \\ \cmidrule(r){2-4}
&  2.  & Human in the loop & Scenarios in which it is unsure whether on interacts with a machine or person. \\ \cmidrule(r){2-4}
&  3.  & Humanness & Mapping of human traits onto technologies, i.e. CUIs. \\ \cmidrule(r){2-4}
&  4.  & Uncanny Valley & Artificial traits that may make users feel uneasy, revulsion, and discomfort when experiencing it. \\ \cmidrule(r){2-4}
&  5.  & Unnatural interactions & Interactions with CUIs do not feel as natural as regular conversation or interaction between humans.\\ \hline
\parbox[t]{1mm}{\multirow{-10}{*}{\rotatebox[origin=c]{90}{Anthropomorphism}}} &  &  & \\

&  6.  & CUIs doing peoples' jobs & Interactions that replace real world jobs such as customer service. This may lead to anthropomorphism. \\ \cmidrule(r){2-4}
&  7.  & Designing voices & Development of speech synthesis for a certain goal, be it humanness or simply task oriented. \\ \cmidrule(r){2-4}
&  8.  & Designing for emotions and social proof & Interfaces that aim to invoke specific emotions or a pressured feeling to follow a set lead. \\ \cmidrule(r){2-4}
&  9.  & Speech vs. text differences & Interactions may differ between voice and text based interfaces. For example visibility of necessary information on the UI level.  \\ \hline
\parbox[t]{1mm}{\multirow{-11}{*}{\rotatebox[origin=c]{90}{CUI Characteristics}}} &  &  & \\ 

&  10. & Capability limitations	& Lack of options due to implementation restrict certain usage demands from users and are thus not meeting their expectations. \\ \cmidrule(r){2-4}
&  11. & Setting false expectations	& Interaction and results may not meet with users' objectives. \\ \cmidrule(r){2-4}
&  12. & Technological limitations & Lack of options due to technological constraints that restrict certain usage demands from users and are thus not meeting their expectations. \\ \cmidrule(r){2-4}
&  13. & Usage frustration & Interactions that are unnecessarily complicated and create a nuisance for users. This may also be result of false expectations. \\ \cmidrule(r){2-4}
&  14. & CUI vs. GUI differences & Situations where designers cannot simply rely on prior experience with GUI technologies. \\ \hline
\parbox[t]{1mm}{\multirow{-12}{*}{\rotatebox[origin=c]{90}{CUI Flaws \& Limitations}}} &  &  & \\

 \end{tabular}
\end{table*}

\newpage

\begin{table*}[h]
\centering

\begin{tabular}{p{.08\textwidth} p{.03\textwidth} p{.25\textwidth} p{.52\textwidth}}
\toprule
\multicolumn{1}{c}{\textbf{Category}} & \multicolumn{1}{c}{\textbf{No.}} & \multicolumn{1}{c}{\textbf{Code}} & \multicolumn{1}{c}{\textbf{Description}}\\ \hline

&  15. &  Applying known dark pattern strategies &  Adopting traditional and described dark pattern strategies and transferring them onto CUI devices. \\ \cmidrule(r){2-4}
&  16. & Coercion of users & Steering or guiding people's decision-making to one's advantage. \\ \cmidrule(r){2-4}
&  17. & Dark pattern evolution and adaptation & Novel changes to dark patterns to overcome users' awareness. \\ \cmidrule(r){2-4}
&  18. & Disparate treatment of users & Treating certain cohorts of users differently than others, i.e. offering/restrciting certain functionality depending on the location or native language. \\ \cmidrule(r){2-4}
&  19. & Manipulation of users &  Willingly taking the risk to harm them in order to gain an advantage. \\ \cmidrule(r){2-4}
&  20. & Obscuring behaviour &  Instances where it is not inherently clear to the user why a CUI does something. \\ \cmidrule(r){2-4}
&  21. & Unintentional/situational CUI dark pattern & Accidentally problematic designs that fit under the umbrella of the dark pattern definition, even if not purposefully implemented. \\ \cmidrule(r){2-4}
&  22. & User burdens & Instances were users face unnecessary obstacles they need to overcome. \\ \hline
\parbox[t]{1mm}{\multirow{-17}{*}{\rotatebox[origin=c]{90}{Dark Pattern Strategies}}} &  &  & \\

&  23. & Cultural and research lag & Most development of CUI systems is done in industry leading to academia not being able to address certain issues before they arise. \\ \cmidrule(r){2-4}
&  24. & Lack of communication between stakeholders & Communication between any combination of users, practitioners, and researchers may be almost non-existent. \\ \cmidrule(r){2-4}
&  25. & Lack of ethics & Addressing ethical concerns when it comes to CUIs and participants' viewpoints. \\ \cmidrule(r){2-4}
&  26. & Lack of guidelines and regulations & Comments on missing standards to comply to or rely on when it comes to use or develop CUIs. \\ \hline
\parbox[t]{1mm}{\multirow{-11}{*}{\rotatebox[origin=c]{90}{Neglect}}} &  &  & \\

&  27.  & Complicated interaction  & While some functionality is quite easy to control, certain others, for example setting one's privacy settings, is unnecessarily difficult to do. \\ \cmidrule(r){2-4}
&  28.  & Opportunities for dark patterns & Some designs which are harmless in most contexts may turn unethical in specific situations. \\ \cmidrule(r){2-4}
&  29. & Persuading users & Influencing users' behaviour through certain design elements. \\ \cmidrule(r){2-4}
&  30. & Situational contexts for interactions & Certain CUI contexts that may result in opportunities for dark patterns but not necessarily. They could also simply lead to frustration and bad user experience. \\ \hline
\parbox[t]{1mm}{\multirow{-11}{*}{\rotatebox[origin=c]{90}{Nudges}}} &  &  & \\
 
\end{tabular}
\end{table*}

\newpage

\begin{table*}[t]
\centering

\begin{tabular}{p{.08\textwidth} p{.03\textwidth} p{.25\textwidth} p{.52\textwidth}}
\toprule
\multicolumn{1}{c}{\textbf{Category}} & \multicolumn{1}{c}{\textbf{No.}} & \multicolumn{1}{c}{\textbf{Code}} & \multicolumn{1}{c}{\textbf{Description}}\\ \hline

&  31. & (In-)transparency of information & Certain information is not always present or easily accessible to all users. \\ \cmidrule(r){2-4}
&  32. &  Privacy concerns & Not all handling of user data is clear while some worry that critical data is shared such as emotions/tonation in voice. \\ \cmidrule(r){2-4}
&  33. &  Privacy paradox & Incongruence between users' privacy concerns and taken actions to safeguard.\\ \hline
\parbox[t]{1mm}{\multirow{-7}{*}{\rotatebox[origin=c]{90}{Trust}}} &  &  & \\

&  34. &  Elderly people & Older people tend to lack confidence or technological literacy. \\ \cmidrule(r){2-4}
&  35. &  Emotional voice of users & Anticipation of angry versus happy prompting of voice based CUIs may lead to distrusting CUI systems that use such information. \\ \cmidrule(r){2-4}
&  36. &  Juveniles or technological naive & Especially children who cannot understand the consequences of ther choices when interacting with CUIs. \\ \cmidrule(r){2-4}
&  37. &  Locational or regional limitations & Varying choices depending on users' localisation. \\ \cmidrule(r){2-4}
&  38. &  Particularly vulnerable people or otherly & This group may contain distinct but similarily vulnerable people such as juveniles, elderly, or people with disabilities. \\ \cmidrule(r){2-4}
&  39. &  People with disabilities & All people who have disabilities may struggle when using CUI systems. \\ \cmidrule(r){2-4}
&  40. &  Second language or dialect or accent issues & Users experience problems and disparate treatment when speaking with a strong accent or are not fluent in the English language. \\ \cmidrule(r){2-4} 
&  41. &  Technological literacy & While some users have a background in technology and understand new interfaces, others lack this knowledge and may be more vulnerable to deceptive strategies.\\ \cmidrule(r){2-4}
&  42. &  User expectations & Users beliefs in a system and how it acts when engaged. Does not necessarily meet a CUIs capabilities. \\ \cmidrule(r){2-4}
&  43. &  User safeguarding & Actions or measures that users take to protect themselves or limit possible harm. \\ \cmidrule(r){2-4}
&  44. &  Users changing behaviour & After a failed interaction, users adopt new strategies when engaging with a system.\\ \hline
\parbox[t]{1mm}{\multirow{-25}{*}{\rotatebox[origin=c]{90}{User Characteristics}}} &  &  & \\

&  45. & Practitioner objectives & Intended functionalities that enable CUIs to solve specific tasks. \\ \cmidrule(r){2-4}
&  46. & Speculation of future CUI technology & Ideas and opinions for how CUI systems may evolve in the future, whether to the positive or negative. \\ \hline
\parbox[t]{1mm}{\multirow{-6}{*}{\rotatebox[origin=c]{90}{Misc.}}} &  &  & \\
 
\end{tabular}
\caption{Inductive codebook table containing 46 individual codes and their descriptions.}
\end{table*}
